# Supplementary material for: Polynomial 2D Green Coordinates for High-order Cages
Source: arXiv:2408.06831 source file (2025-05-27)
Supplement: Supplementary file 1 [file appendix.tex]

\section{The Formulation of $\alpha_i^{n_s}$ and  $\beta_i^{n_s}$}
 When $n_s=2$, we have:
 \begin{equation}
     \alpha_0=(c_0-\eta)c_1^{\perp}, \alpha_1=2(c_0-\eta)c_2^{\perp}, \alpha_2=c_1 \cdot c_2^{\perp}.
 \end{equation}
 \begin{equation}
 \begin{aligned}
     &\beta_0=(c_0-\eta)c_1, \beta_1=\|c_1\|^2+2 (c_0-\eta)\cdot c_2,\\
     &\beta_2=3 c_1\cdot c_2, \beta_3=2 \|c_2\|^2.
\end{aligned}
 \end{equation}

 When $n_s=3$, we have:
 \begin{equation}
 \begin{aligned}
     &\alpha_0=(c_0-\eta)c_1^{\perp}, \alpha_1=2(c_0-\eta)c_2^{\perp},\\
     &\alpha_2=3(c_0-\eta)\cdot c_3^{\perp}+\frac{4}{3}c_1 c_2^{\perp}+\frac{1}{3}c_2 c_3^{\perp},\\
     &\alpha_3=2c_1 c_3^{\perp}, \alpha_4=c_2 c_3^{\perp}.
\end{aligned}
 \end{equation}
 \begin{equation}
 \begin{aligned}
     &\beta_0=(c_0-\eta)c_1, \beta_1=\|c_1\|^2+2 (c_0-\eta)\cdot c_2,\\
     &\beta_2=3 c_1\cdot c_2+3(c_0-\eta)c_3, \beta_3=2 \|c_2\|^2+4 c_1 c_3,\\
     &\beta_4=5 c_2 c_3, \beta_5=3 \|c_3\|^2.
\end{aligned}
 \end{equation}
